# Supplementary material for: Differential Flatness of Quadrotor Dynamics Subject to Rotor Drag for Accurate Tracking of High-Speed Trajectories
Source: arXiv:1712.02402 source file (2018-03-28)
Supplement: Supplementary file 1 [file appendices.tex]

\section{Incorrectnesses in Original Differential Flatness Derivation} \label{sec:mellinger_mistakes}
 
The work presented in~\cite{Faessler18ral} extends the work of~\cite{Mellinger11icra}, which can be considered the first paper that proves differential flatness for quadrotors without considering rotor drag.
However, we would like to point out two incorrectnesses found in~\cite{Mellinger11icra} that might be confusing when comparing it to our derivations.
For this, we use red color to refer to equations in~\cite{Mellinger11icra}.
Note that in this work we are using a different index convention, i.e., we denote the rotation rates of e.g. $\bfr$ with respect to $\wfr$ as $\vect{\bodyrates}{}{\wfr \bfr}$ whereas it is denoted as $\vect{\bodyrates}{}{\bfr \wfr}$ in~\cite{Mellinger11icra} but in this section, we adopt their convention when referring to their equations.
\newline\newline
The first incorrectness in~\cite{Mellinger11icra} is due to a confusion of the representation of vectors in world or body coordinates (see Section~\ref{sec:vector_derivatives} for details).
In equation~{\color{red} (7)} the derivative of equation~{\color{red} (3)} is computed as
\begin{equation}
	\color{red}
	m \dot{\acc} = \dot{u}_1 \vect{z}{}{\bfr} + \vect{\bodyrates}{}{\bfr \wfr} \times u_1 \vect{z}{}{\bfr} . \label{eq:mellinger_wrong_derivative}
\end{equation}
However, equation~{\color{red} (3)} including $\vect{z}{}{\bfr}$ is represented in world coordinates.
By taking its derivative, we get
\begin{align}
	m \dot{\acc} &= \dot{u}_1 \vect{z}{}{\bfr} + u_1 \vectdot{z}{}{\bfr} \\
	&= \dot{u}_1 \vect{z}{}{\bfr} + u_1 \ori{} \hat{\bodyrates} \vect{\uvec}{}{z} .
\end{align}
The fallacy in~\eqref{eq:mellinger_wrong_derivative} is that $\vectdot{z}{}{\bfr}$ is computed as if $\vect{z}{}{\bfr}$ was represented in body coordinates (c.f.~\eqref{eq:body_vec_deriv_body}) but it is represented in world coordinates and hence its derivative is ${\vectdot{z}{}{\bfr} = \ori{} \hat{\bodyrates} \vect{\uvec}{}{z}}$, (c.f.~\eqref{eq:body_vec_deriv_world}).
However, by chance, the correct roll and pitch rates are obtained in~\cite{Mellinger11icra} since the projections of ${\color{red} \vect{\bodyrates}{}{\bfr \wfr} \times \vect{z}{}{\bfr}}$ and ${\ori{} \hat{\bodyrates} \vect{\uvec}{}{z}}$ onto the $\vect{x}{}{\bfr}$ and $\vect{y}{}{\bfr}$ axes are equal.
Note that when taking the second derivative of equation~{\color{red} (3)} as done in~\cite{Mellinger11icra} and computing the angular accelerations from that, unlike for the body rates, would not result in correct values anymore.
\newline\newline
The second incorrectness in~\cite{Mellinger11icra} in the same section in the computation of the third component of the body rates.
It is stated that \emph{"the third component $r$ is found by simply writing ${\vect{\bodyrates}{}{\bfr \wfr} = \vect{\bodyrates}{}{\bfr \cfr} + \vect{\bodyrates}{}{\cfr \wfr}}$ and observing that $\vect{\bodyrates}{}{\bfr \cfr}$ has no $\vect{z}{}{\bfr}$ component"}, which is not correct, i.e., generally ${\vect{\bodyrates}{}{\bfr \cfr} \cdot \vect{z}{}{\bfr} \neq 0}$.
Based on this incorrect assumption, the third component of the body rates is then computed as
\begin{equation}
	\color{red}
	r = \vect{\bodyrates}{}{\cfr \wfr} \cdot \vect{z}{}{\bfr} = \dot{\heading} \vect{z}{}{\wfr} \cdot \vect{z}{}{\bfr} \label{eq:mellinger_wrong_yaw_rate}
\end{equation}
but for
\begin{equation}
	\vect{\bodyrates}{}{\bfr \wfr} = \vect{\bodyrates}{}{\bfr \cfr} + \vect{\bodyrates}{}{\cfr \wfr}
\end{equation}
to hold, all vectors must be expressed in the same coordinate frame, which in this case has to be the $\bfr$ frame since the body rates $\vect{\bodyrates}{}{\bfr \wfr}$ are expressed in body coordinates.
Conversely, ${\vect{\bodyrates}{}{\cfr \wfr} = \dot{\heading} \vect{z}{}{\wfr}}$ as used in~\eqref{eq:mellinger_wrong_yaw_rate} is only valid if $\vect{\bodyrates}{}{\cfr \wfr}$ was expressed in world coordinates, which is not the case.
Similarly, the angular accelerations are computed incorrectly.
The necessary third constraint for computing the correct body rates is \eqref{eq:yaw_rate}.
